# Supplementary material for: Fundamental laws of chiral band crossings: local constraints, global constraints, and topological phase diagrams
Source: arXiv:2303.01477 source file (2023-03-02)

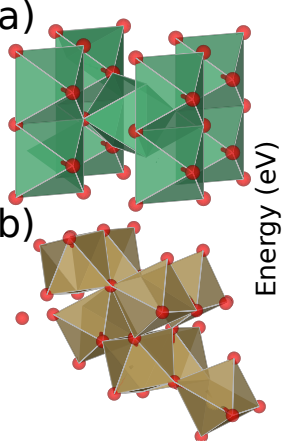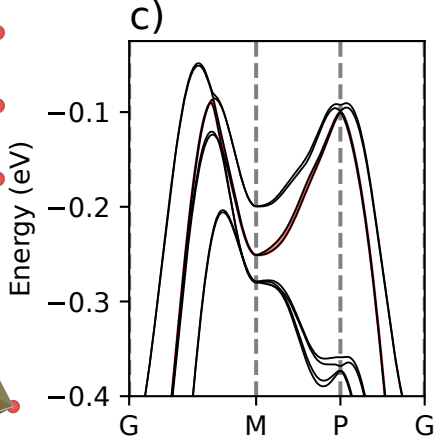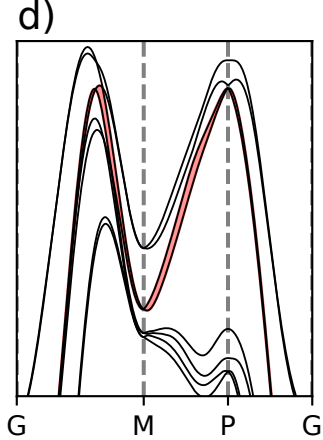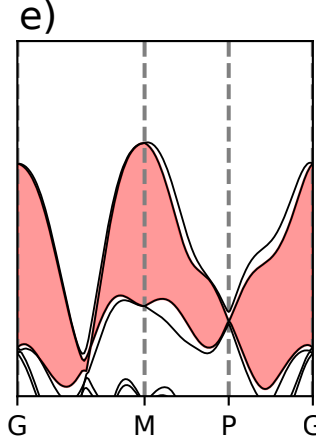

Supplement: Supplementary file 1 [file tao2_appendix.pdf]
